# Supplementary material for: Orbital magnetization of a metal is not a bulk property in the mesoscopic regime
Source: arXiv:2309.03957 source file (2024-04-30)
Supplement: Supplementary file 1 [file supp.pdf]

# Supplement to "Orbital magnetization of a metal is not a bulk property in the mesoscopic regime"

Kevin Moseni[1] and Sinisa Coh[1,2]

[1] *Materials Science and Engineering, University of California Riverside, Riverside, CA 92521, USA*
[2] *Mechanical Engineering, University of California Riverside, Riverside, CA 92521, USA*

(Dated: April 30, 2024)

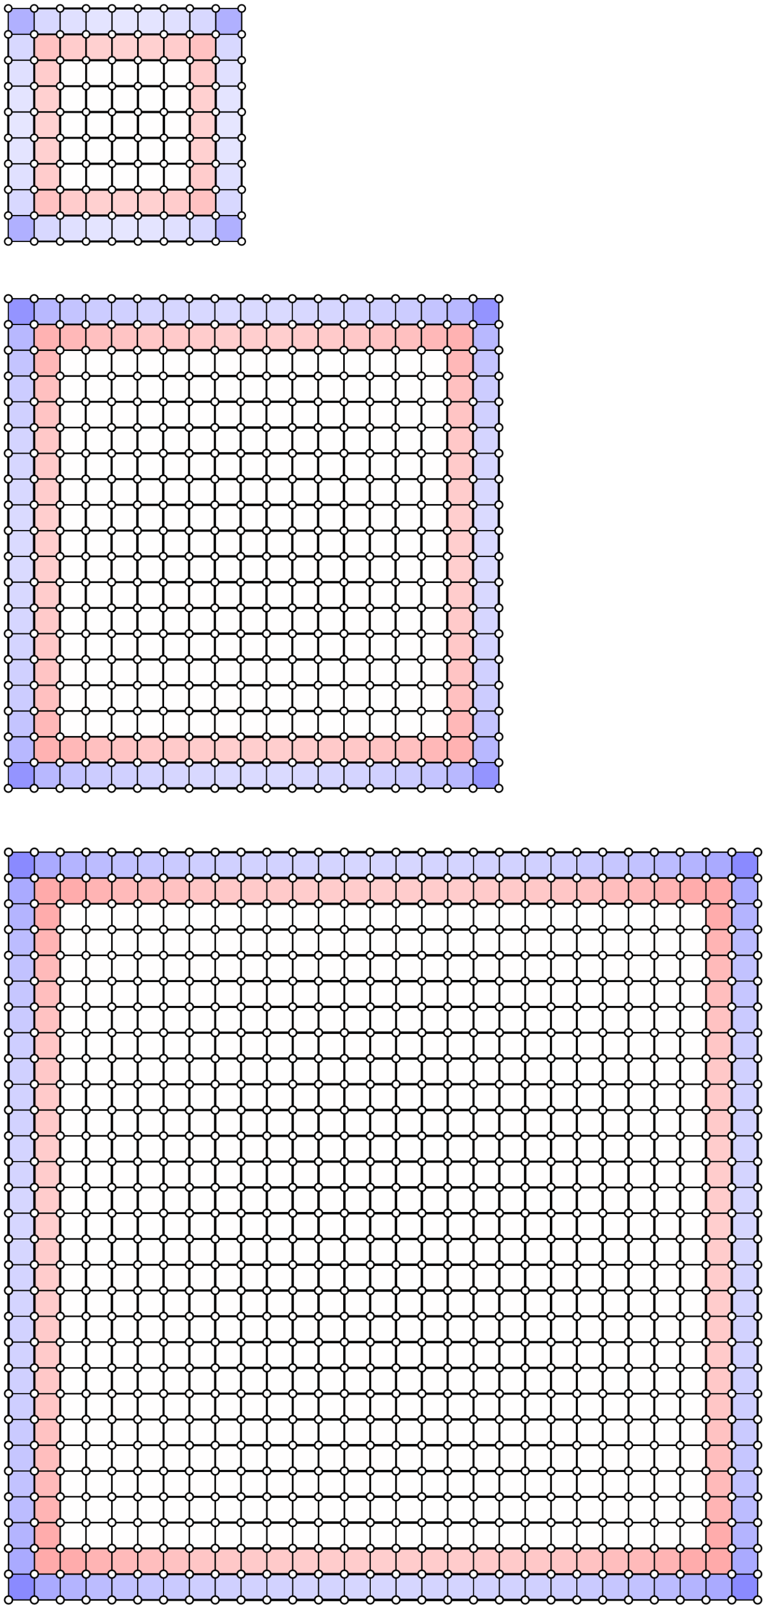

FIG. 1. Sketch of $H = H^{\rm bulk} + V^{\rm edge}$ for $N = 10$, 20, and 30. Small circles represent orbitals $i$. The black lines represent the hopping parameters $H_{ij}$. The thickness of each black line is proportional to $|H_{ij}|$. The variation in the thickness of the black lines is mainly due to $H^{\rm comm}$. For each square, defined with orbitals $i$, $j$, $k$, $l$ with fixed handedness, we compute the complex phase of $H_{ij}H_{jk}H_{kl}H_{li}$ around the square. If the complex phase is positive, we color the square darker shade of blue, and if it is negative, we color the square darker shade of red. Normalization of the color scale is the same in all three panels.

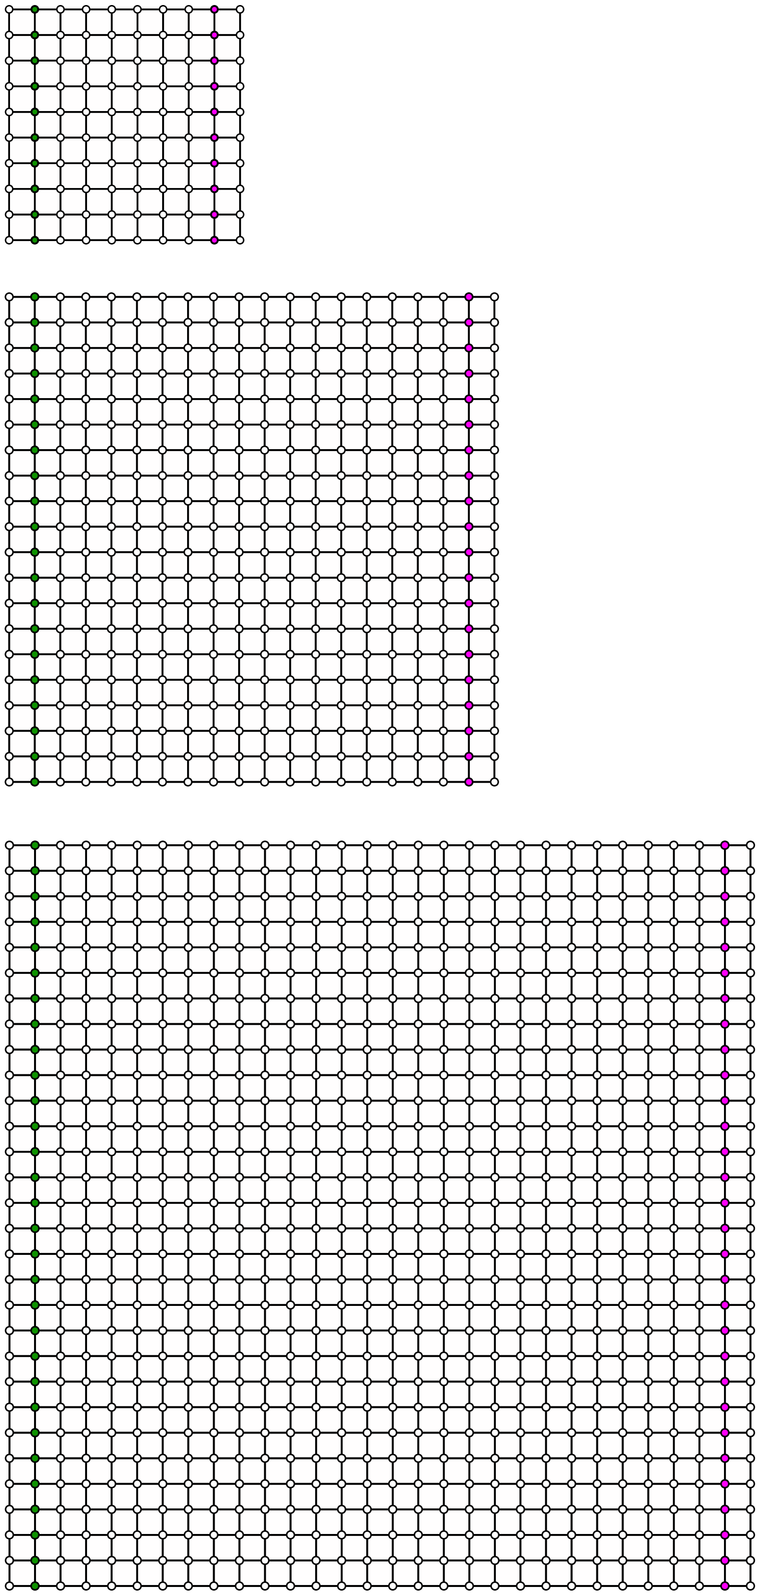

FIG. 2. Sketch of the model using the construction for the electrical dipole $V'^{\mathrm{edge}}$ in analogy to our construction for the magnetic dipole. Small circles represent orbitals. The black lines represent the hopping parameters. Here, in the case of the electrical dipole, all hopping parameters have the same magnitude. The edge perturbation for the dipole moment introduces a constant (independent of $N$) change of the onsite energy at the left and right edge. The different sign of change in the onsite energy on the left versus right edge is indicated with green and purple color.

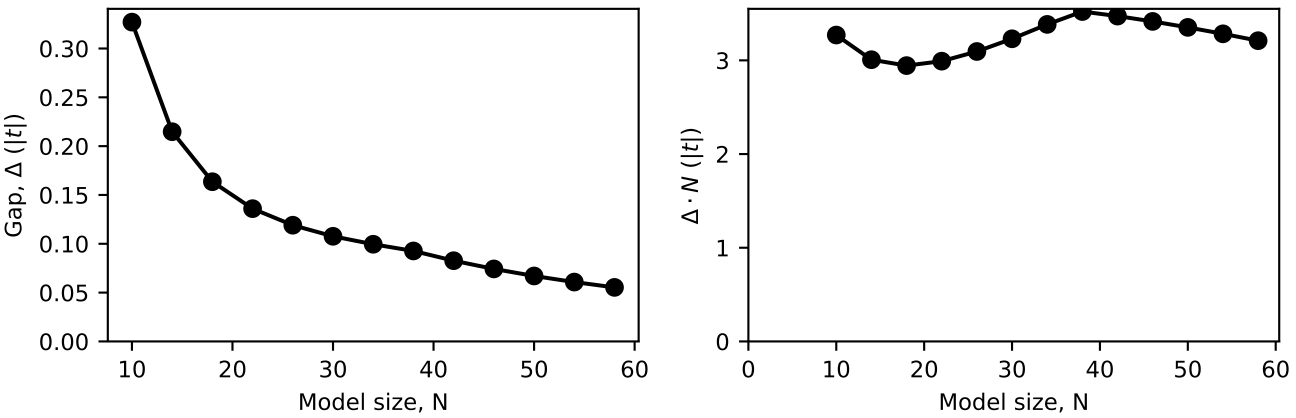


FIG. 3. At $E_{\mathrm{F}} \approx -2.55\,|t|$, our model has a gap of size $\Delta$. We find that $\Delta$ scales as $1/N$ with model size ($N$), and therefore $\Delta \to 0$ when $N \to \infty$, as expected for a metallic system. The data on the plot fits well to $\Delta \approx \frac{3|t|}{N}$
